# Supplementary material for: A Multimodal Vision Foundation Model for Clinical Dermatology
Source: arXiv:2410.15038 source file (2025-04-13)

**a**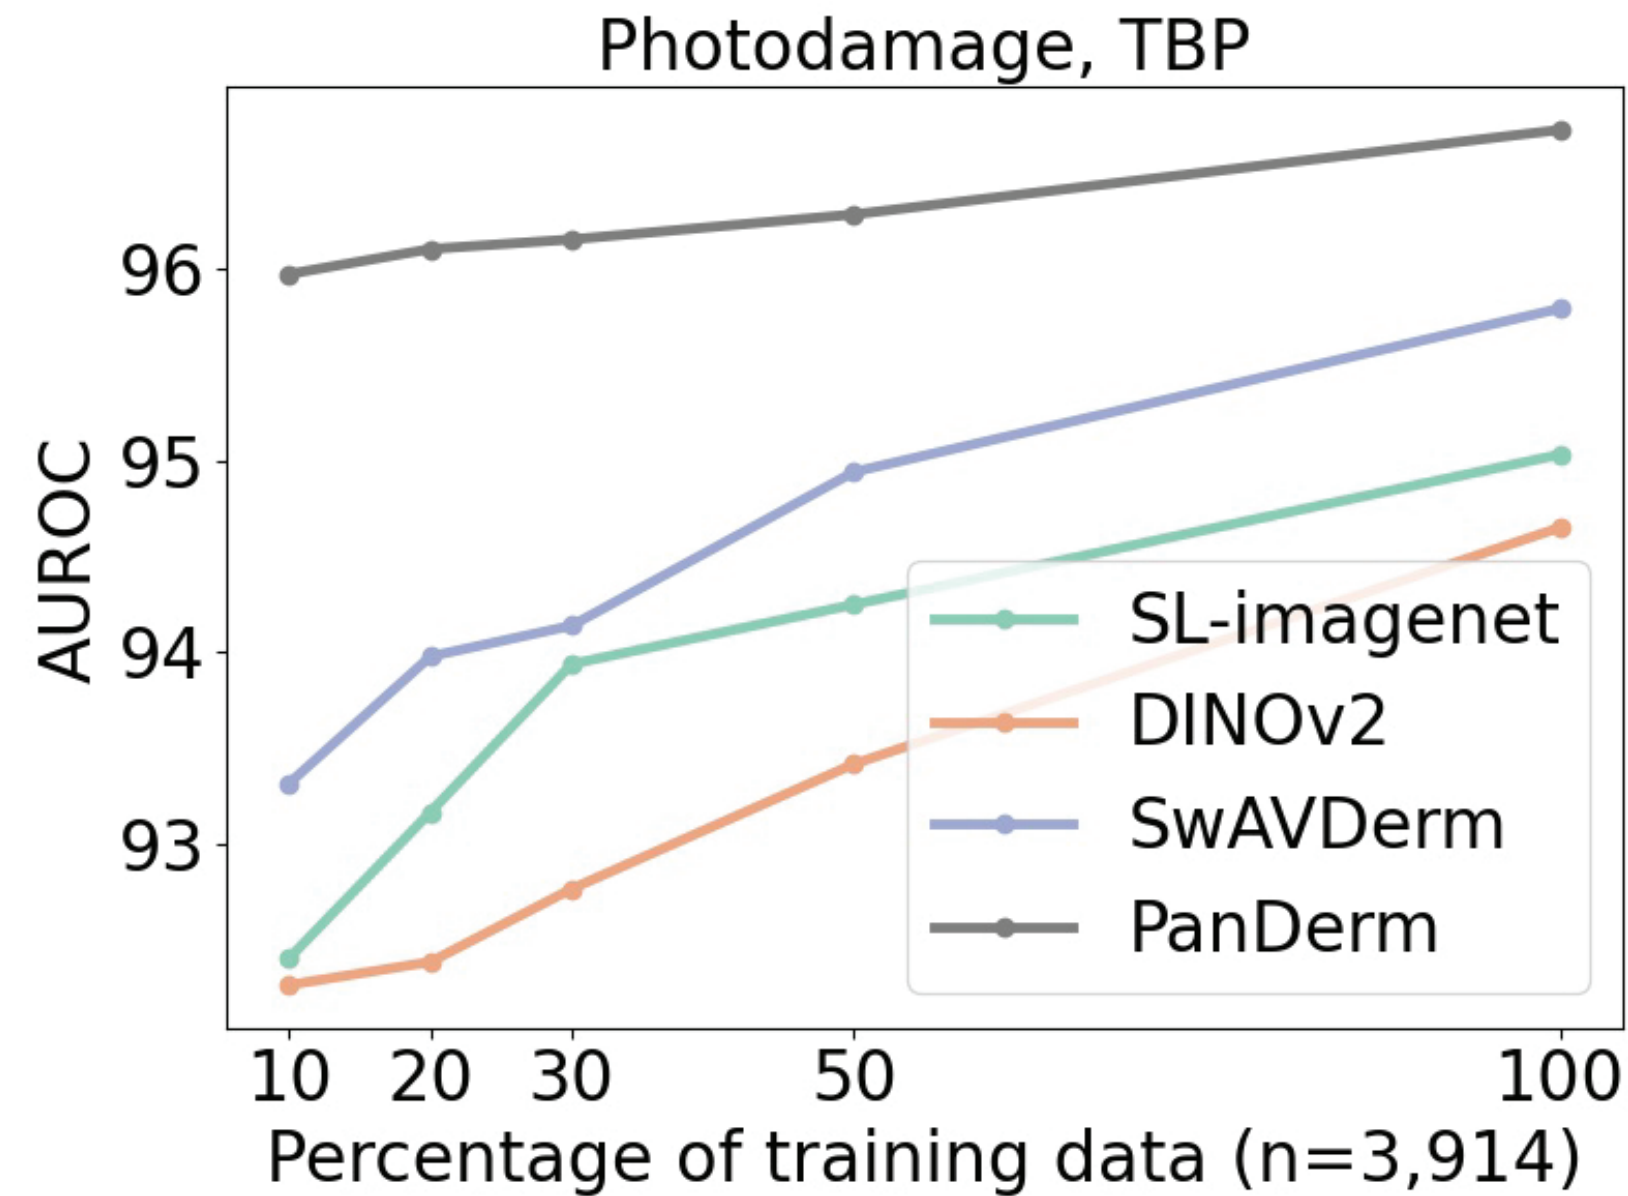**b**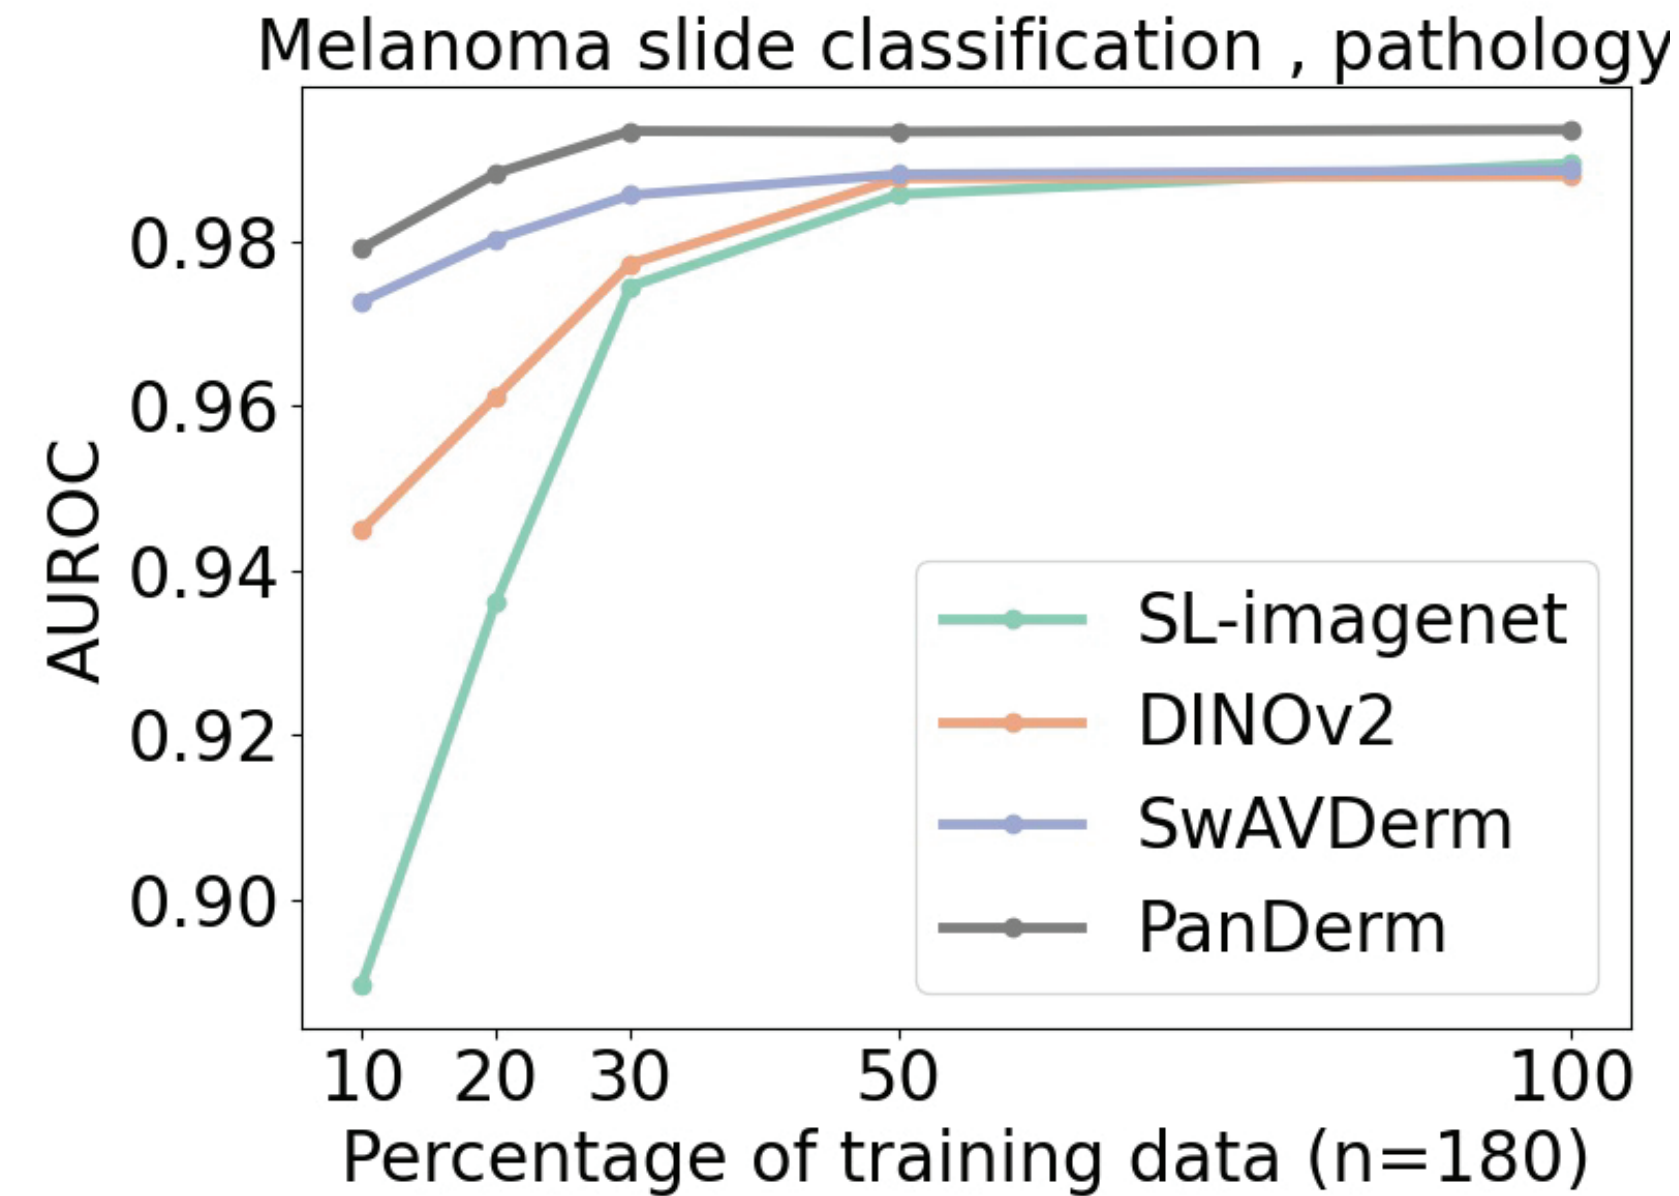

Supplement: Supplementary file 1 [file supp_fig3.pdf]
